# Supplementary material for: Zemi: Learning Zero-Shot Semi-Parametric Language Models from Multiple Tasks
Source: arXiv:2210.00185 source file (2023-05-23)
Supplement: Supplementary file 1 [file additional_analysis.tex]

% \subsection{Why semi-parametric multitask training works?}
% \label{sec:additional_ablation}

\begin{wrapfigure}{r}{7cm}
\vspace{-10pt}
% \begin{figure}[thb]
\begin{minipage}{0.51\textwidth}
    \centering
    \includegraphics[width=\textwidth]{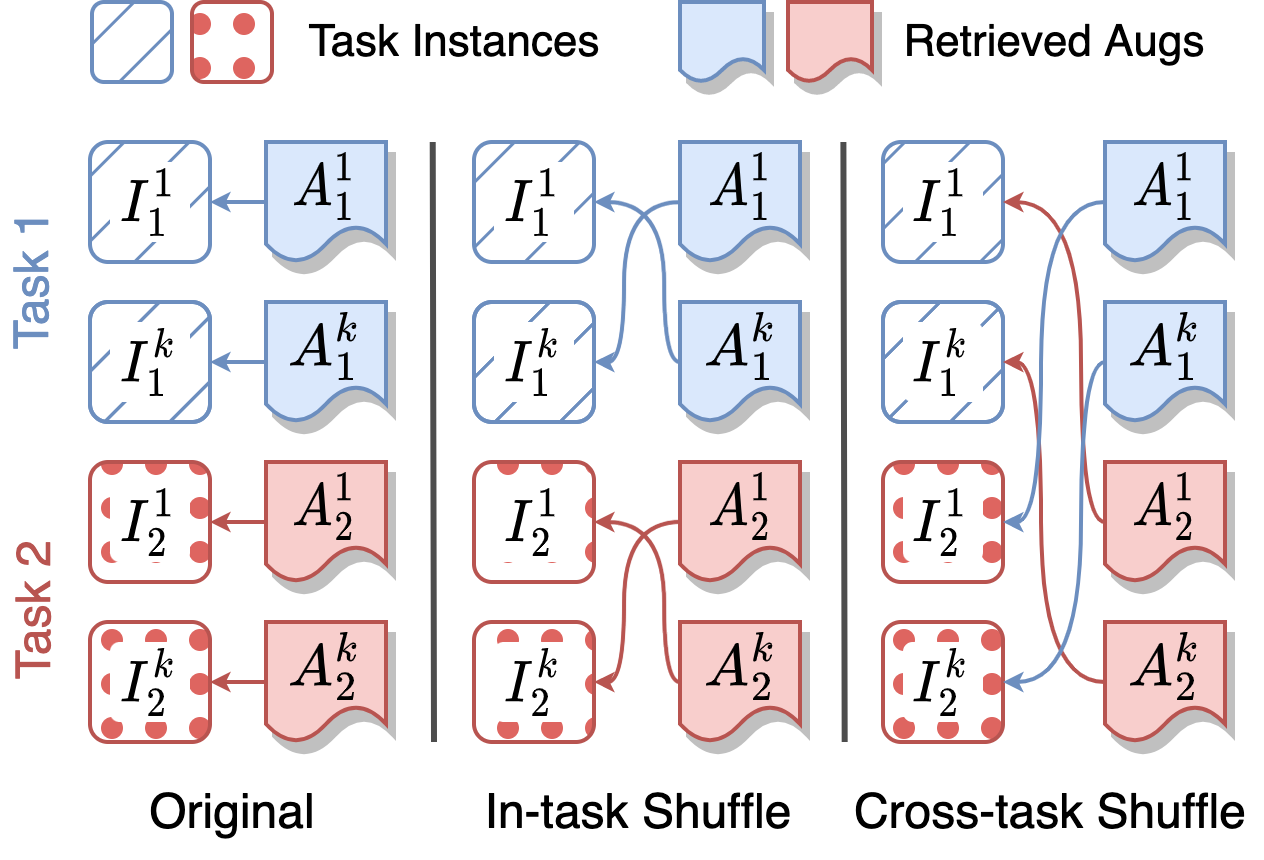}
    \vspace{-15pt}
    \caption{Augmentation shuffling strategies.}
    % Detailed results on each task can be found in Table~\ref{table:aug_shuffle_single_task},\ref{table:aug_shuffle_multitask}. }
    \label{fig:shuffle_strategy}
\end{minipage}
\vspace{-5pt}
\end{wrapfigure}

In Table~\ref{table:main_result}, we show that existing augmentation fusion methods cannot achieve visible positive gain due to the noisy retrieval as visualized in Appendix~\ref{sec:retrieval_examples}. In contrast, \ours{} is able to achieve significant improvement by leveraging the noisy retrieved augmentations. In this section, we aim to further investigate \textit{what is the key benefit of the retrieval augmentation that helps improve zero-shot task generalization}.
% In this section we aim to investigate why \textit{semi-parametric multitask training} helps further improve zero-shot task generalization compared with \textit{parametric multitask training}. The main goal is to explore what kind of additional information derived from the retrieval that is of most importance towards effective zero-shot generalization. 
To this end, we design an additional ablation study on the retrieval augmentation. We introduce two types of perturbations on the original retrieved augmentations, i.e., \textbf{in-task shuffle} and \textbf{cross-task shuffle}. As illustrated in Figure~\ref{fig:shuffle_strategy}, for in-task Shuffle, during both training and evaluation, we replace the augmentation of each instance with a randomly picked retrieved augmentation from another instance \textbf{within the same task}. For cross-task shuffle, we replace the augmentation of each instance with a randomly picked retrieved augmentation from \textbf{a different task} in the entire training and evaluation mixtures. 
Table~\ref{table:aug_shuffle_multitask} shows the averaged relative gain against the \textit{No Aug} baseline.

% \begin{table*}[!hbt]
\begin{wraptable}{r}{7cm}
\vspace{-10pt}
\small
\centering
\setlength\tabcolsep{3pt}
% \setlength\extrarowheight{1pt}
% \begin{tabularx}{\linewidth}{l|CCCC}
\begin{tabular}{c | c || c | c | c }
\toprule

\multirow{2}{*}{\textbf{Task}} &
\multirow{2}{*}{\textbf{No Aug}}&
\multirow{1}{*}{\textbf{\ours{}}}&
\multirow{1}{*}{\textbf{In-task}}&
\multirow{1}{*}{\textbf{Cross-task}}
\\
& & \textbf{Original} & \textbf{Shuffle} & \textbf{Shuffle}
\\
\midrule
OBQA    & \;36.64  &  35.55  & \,36.02  & \,34.49 \\
Piqa    & \;60.24  &  59.23  & \,60.00  & \,59.30 \\
RT      & \;64.11           &  68.58   & \,63.04   & \,71.97\\
CB      & \;41.46           &  50.05    & \,47.92 & \,42.08\\
COPA    & \;68.46           &  63.57   & \,64.94   & \,70.41  \\
WiC     & \;49.92           &  49.56  & \,50.47  & \,52.40 \\
HSwag   & \;27.97           &  29.68   & \,29.09 & \,29.49 \\

\midrule
Rel $\Delta$ Avg    & \;0.00   & +3.04   & \,+1.77  & \,+2.80 \\
% Median $\Delta$ & 0.00 & 0.00 & +1.70 & +0.47 & +1.65 & +0.47 & +1.43 & +0.78 & +1.69 & +0.55\\
\bottomrule
% \end{tabularx}
\end{tabular}

\caption{Impact of perturbing augmentations on semi-parametric multitask prompted training to zero-shot task generalization.}
\label{table:aug_shuffle_multitask}
\end{wraptable}

 Our main observation is that \textbf{capturing task-level correlation} is the key factor towards effective retrieval augmentation. First, we observe that doing in-task or cross-task shuffle can hurt the performance, which is intuitive since the shuffling weakens the instance-level correlation between the input and the augmentations. However, interestingly, we find that cross-task shuffle has a smaller negative impact on the performance than the in-task shuffle. This is showing that capturing the overall task-level correlation between the input instances and the augmentations is more important than capturing instance-level correlation. Thus, from a data augmentation perspective, we hypothesis that augmenting multitask training with retrieved documents from a large-scale task-agnostic corpus, despite being noisy, can encourage the model to learn generalizable abilities for solving various kinds of tasks instead of one specific task.

% capturing the general information of the current 
% while in the multi-task setting the observation reversed. This is showing that if the optimization objective is a single task, the key requirement of the augmentations is to capture the general \textbf{task-level features of the current task}. Intuitively, if our optimization objective is a wide range of tasks, the key to effective augmentation becomes capturing the \textbf{overall task-level features of multiple tasks}.
